# Supplementary material for: A Walk in Facebook: Uniform Sampling of Users in Online Social Networks
Source: arXiv:0906.0060 source file (2011-06-17)
Supplement: Supplementary file 1 [file appendix.tex]

\section*{Appendix: Correctness of UNI Sampling}
\label{sec:UNIsampling}
\noindent {\bf Proposition:}
UNI (defined in Section \ref{sec:uni}, as uniform sampling of 32-bit IDs and discarding the non existing ones) yields a uniform sample of the {\em existing (allocated)} user IDs in \facebook for {\em any allocation policy} ({\em e.g.,} even if the userIDs are not evenly allocated in the 32-bit address space).
\vspace{10pt}

\noindent {\bf Proof.}
Denote by $U$ the set of all possible user IDs, {\em i.e.,} the set of all integers in  $[0,2^{32}-1]$. Let $A\subset U$ be the set of allocated user IDs in \facebook. We would like to sample the elements in $A$ uniformly, {\em i.e.,} with pdf $f_A(x) = \frac{1}{|A|}\sum_{y\in A} \delta(y)$,
where $\delta(y)$ is the Dirac delta.
The difficulty is that we do not know the allocated IDs $A$ beforehand. However, we are able to verify whether id $x$ exists ($x\in A$) or not, for any $x$.

   To achieve this goal, we apply rejection sampling \cite{leon-garcia} as follows. Choose uniformly at random an element from $U$ (which is easy), {\em i.e.,} with pdf
$f_U(x) = \frac{1}{|U|}\sum_{y\in U} \delta(y)$.
 Let $K=\frac{|U|}{|A|}$ s.t. $f_A(x)\leq K\cdot f_U(x)$ for any $x$. Now, draw $x$ from $f_U(x)$ and accept it with probability $\frac{f_A(x)}{K\cdot f_U(x)} = 1_{x\in A},$
{\em i.e.}, always if $x\in A$ (ID $x$ exists/is allocated) and never if $x\notin A$ (ID $x$ is not allocated).
The resulting sample follows the distribution $f_A(x)$, {\em i.e.,} is taken uniformly at random from $A$ (the set of {\em allocated} user IDs).
\hfill $\Box$

The above is just a special case of {\em rejection sampling} \cite{leon-garcia}, when the distribution of interest is uniform. It is presented here for completeness, given the importance of UNI sampling as ``ground truth'' in the paper.
